# Supplementary material for: ProtoMedX: Towards Explainable Multi-Modal Prototype Learning for Bone Health Classification
Source: arXiv:2509.14830 source file (2025-10-09)
Supplement: Supplementary file 1 [file X_suppl.tex]

\clearpage
\setcounter{page}{1}
\maketitlesupplementary

\section{Rationale}
\label{sec:rationale}
Having the supplementary compiled together with the main paper means that:
\begin{itemize}
\item The supplementary can back-reference sections of the main paper, for example, we can refer to \cref{sec:intro};
\item The main paper can forward reference sub-sections within the supplementary explicitly (e.g. referring to a particular experiment); 
\item When submitted to arXiv, the supplementary will already included at the end of the paper.
\end{itemize}
To split the supplementary pages from the main paper, you can use \href{https://support.apple.com/en-ca/guide/preview/prvw11793/mac#:~:text=Delete%20a%20page%20from%20a,or%20choose%20Edit%20%3E%20Delete).}{Preview (on macOS)}, \href{https://www.adobe.com/acrobat/how-to/delete-pages-from-pdf.html#:~:text=Choose%20%E2%80%9CTools%E2%80%9D%20%3E%20%E2%80%9COrganize,or%20pages%20from%20the%20file.}{Adobe Acrobat} (on all OSs), as well as \href{https://superuser.com/questions/517986/is-it-possible-to-delete-some-pages-of-a-pdf-document}{command line tools}.

\subsection{Pre-Processing}

There are at times significant visual differences between images. The main cause of this is due to patients receiving different dose levels during their scans, due to the size differences of the patients (larger patients requiring a larger dose, compared to smaller patients). While this is a crucial step for the DEXA scanners to produce accurate readings, it makes training and testing machine learning models on these scans more challenging. Most notably, a model may mistakenly focus on intensity variations rather than the structural details of the spine. In this regards, we combined several image processing techniques to assist with image normalisation. Note that the normalisation techniques I employed were applied on a per-image basis, not across the dataset, as this has been shown to be more effective for medical datasets where images can vary widely in brightness\cite{Schmid2023}. \\

\noindent \textbf{Z-score normalisation}
\noindent Otherwise known as standardisation, this technique converts each pixel value to have zero mean and unit variance, helping reduce sensitivity to illumination changes.\\

\[
I' = \frac{I - \mu}{\sigma}
\]

Where \( I' \) is the normalised pixel value, \( I \) is the original pixel value, \( \mu \) is the mean of the image and \( \sigma \) is the standard deviation of the image. \\

\noindent \textbf{Gamma correction}
\noindent This is a non-linear transformation, which adjusts brightness and contrast levels, enhancing details in areas that are either really bright or really dark. \\
\[
I' = 255 \times \left(\frac{I}{255}\right)^\gamma
\]

Where \( I' \) is the gamma-corrected pixel intensity, \( I \) is the original pixel intensity (ranging from 0 to 255), and \( \gamma \) (gamma value) controls the brightness adjustment. \\

\noindent If \( \gamma > 1 \), the image becomes darker, reducing the brightness of already bright regions. If \( \gamma < 1 \), the image becomes brighter, enhancing darker regions. \\

\noindent \textbf{Contrast Limited Adaptive Histogram Equalisation}
\noindent It is not always a good idea in histogram equalisation to consider the global contrast of the image, as it may improve certain regions while losing important details in others. CLAHE addresses this issue by dividing the image into small blocks and applying histogram equalisation to each block individually\cite{OpenCVHistEqualization}. This reduces the risk of losing information through incidental over, or under, exposure. CLAHE has been used successfully on MRIs, sonography, and X-ray images\cite{Singh2017}, so it was a clear choice to use here. \\

\textbf{CAN WE USE THE ACTUAL IMAGES? OR IS THAT TOO CONFIDENTIAL?}

\begin{figure}[htbp]
    \centering
    \begin{subfigure}{0.2\textwidth}
        \centering
        \includegraphics[width=\linewidth]{ICCV2025-Author-Kit/img/normal (1).PNG}
    \end{subfigure}
    \hfill
    \begin{subfigure}{0.2\textwidth}
        \centering
        \includegraphics[width=\linewidth]{ICCV2025-Author-Kit/img/normal (2).PNG}
    \end{subfigure}
    \caption{Two DEXA scans of spines with normal bone health from a public dataset\cite{malik2021osteoporosis} that have used our post processing method.}
\end{figure}

Nevertheless, if patients received scans at different dose levels, there is only so much that can be done through image processing. While broadly across the dataset, there is more visual consistency between the images, some images still vary in brightness, quality, and contrast significantly, which is always going to happen when a dataset grows large enough.

It is for this reason we discourage what other research papers have done, which is converting images into their binary equivelant, as we have found that with messy data, this processing effect does more harm to the results than good, as can be seen in our results and from the demonstration below.

\begin{figure}[htbp]
    \centering
    \begin{subfigure}{0.2\textwidth}
        \centering
        \includegraphics[width=\linewidth]{ICCV2025-Author-Kit/img/Alternative (1).PNG}
    \end{subfigure}
    \hfill
    \begin{subfigure}{0.2\textwidth}
        \centering
        \includegraphics[width=\linewidth]{ICCV2025-Author-Kit/img/Alternative (2).PNG}
    \end{subfigure}
    \caption{Two DEXA scans of spines with normal bone health from a public dataset\cite{malik2021osteoporosis} that have used existing pre-processing techniques.}
\end{figure}

%%%%%%%%%%%%%%%%%%%%%%%%%%%%%%%%%%%%%%%%%%%%%%%%%%%%%%%%%%%%%%%%%%%%%%%%%%%%%%%%%%%%%%%%%%%%%%%%%%%%%%%%%%%%%%%%%%%%%%%%%%%%%%%%%%%%%%%%%%%%%%%%%%%%%%%%%%%%%%%%%%%%%%%%%%%%%%%%%%%%%%%%%%%%%%%%%%%%%%%%%%%
\begin{table*}[ht]
\centering
\begin{tabular}{|l|c|c|c|c|c|c|c|}
\hline
\textbf{Method} & \textbf{Modality} & \textbf{Excl.} & \textbf{Acc.} & \textbf{Prec.} & \textbf{Rec.} & \textbf{F1} & \textbf{AUC} \\
\hline
CrossViT & Vision & Yes & 72.2 & 66.3 & 64.2 & 65.1 & 86.1 \\
CrossViT & Vision & No & \textbf{74.7} & \textbf{69.5} & \textbf{67.7} & \textbf{68.5} & \textbf{88.4} \\
\hline
MLP & Vision & Yes & 70.6 & 64.2 & 64.1 & 64.1 & 84.9 \\
MLP & Vision & No & \textbf{73.2} & \textbf{65.8} & \textbf{66.1} & \textbf{65.9} & \textbf{85.5} \\
\hline
XGBoost & Vision & Yes & 70.6 & 65.0 & 63.6 & 64.2 & 84.6 \\
XGBoost & Vision & No & \textbf{73.2} & \textbf{65.7} & \textbf{66.0} & \textbf{65.9} & \textbf{84.8} \\
\hline
CrossViT & Combined & Yes & 72.5 & 66.6 & 61.7 & 62.9 & 86.6 \\
CrossViT & Combined & No & \textbf{76.2} & \textbf{75.2} & \textbf{64.1} & \textbf{66.2} & \textbf{89.1} \\
\hline
MLP & Combined & Yes & 55.2 & \textbf{70.0} & 57.4 & 51.2 & 84.8 \\
MLP & Combined & No & \textbf{72.3} & 65.3 & \textbf{66.0} & \textbf{65.6} & \textbf{85.1} \\
\hline
\end{tabular}
\caption{Model performance with and without vertebral exclusions across vision-only and combined modalities. Analysis of vertebral exclusions showed minimal impact ($2$ to $3\%$ accuracy difference), validating our preprocessing approach. Misclassification analysis reveals most errors occur at diagnostic boundaries (Normal → Osteopenia: 7 cases, Osteoporosis → Osteopenia: 5 cases), consistent with clinical uncertainty in borderline cases.}
\label{tab:combined-results}
\end{table*}
